# Supplementary material for: Multiscale Modeling of Binary Polymer Mixtures: Scale Bridging in the Athermal and Thermal Regime
Source: arXiv:1008.1038 source file (2010-08-05)
Supplement: Supplementary file 1 [file SupplementalMaterial.pdf]

# I. SUPPLEMENTAL MATERIAL

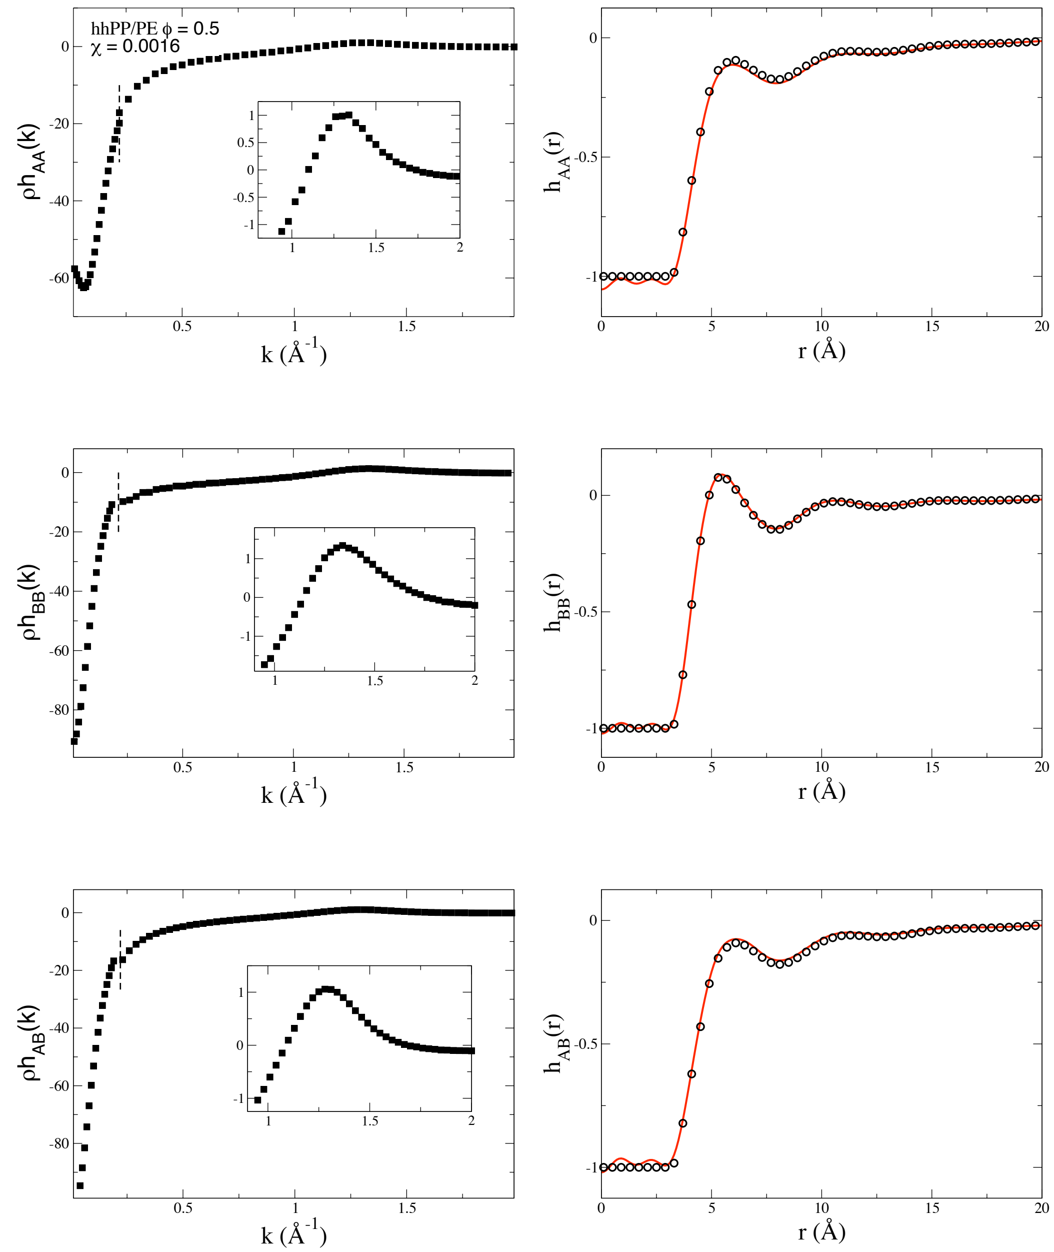


FIG. 1: Multiscale modeling procedure for a thermal mixture of hhPP/PE at $T = 453K$, corresponding to a value of $\chi = 0.0016$ in our mesoscale simulations. The left panel shows the correlation function for AA, BB, and AB components obtained by combining local and large-scale information from independent simulations. The dashed line indicates the place where the two sets of data were combined. The right panel shows the resulting total correlation function in real space (solid red line) as compared with full UA MD simulation (open symbols).

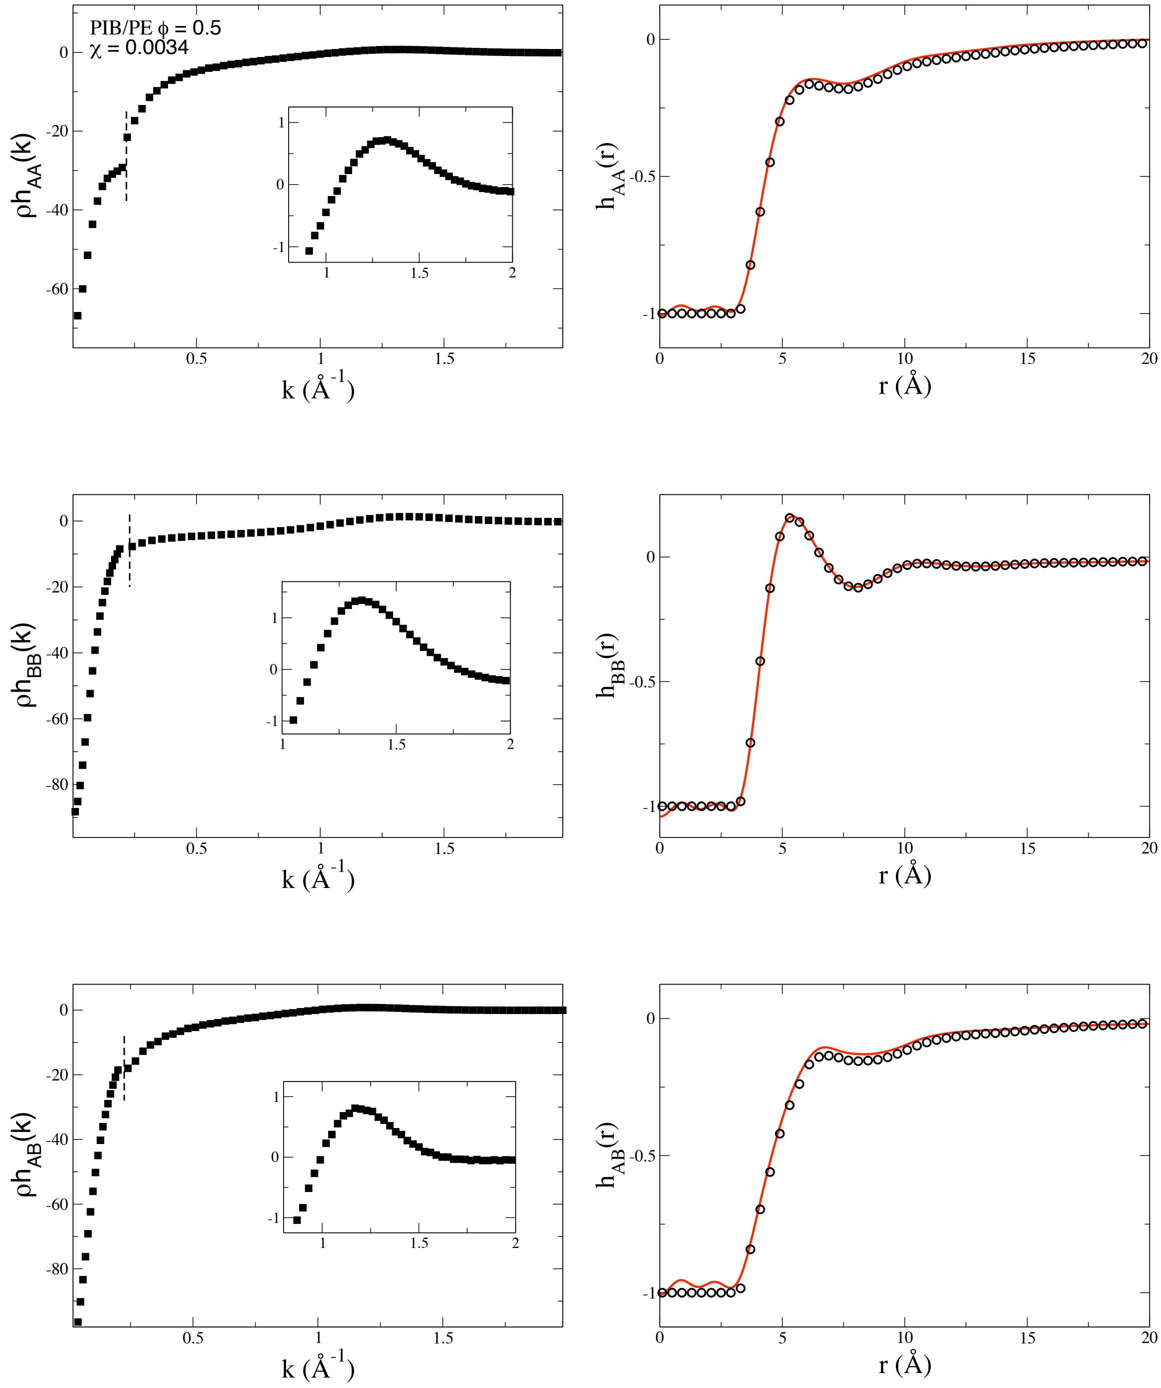


FIG. 2: Same as in Figure 1 except for a thermal mixture of PIB/PE at $T = 453K$, corresponding to a value of $\chi = 0.0034$ in our mesoscale simulations.

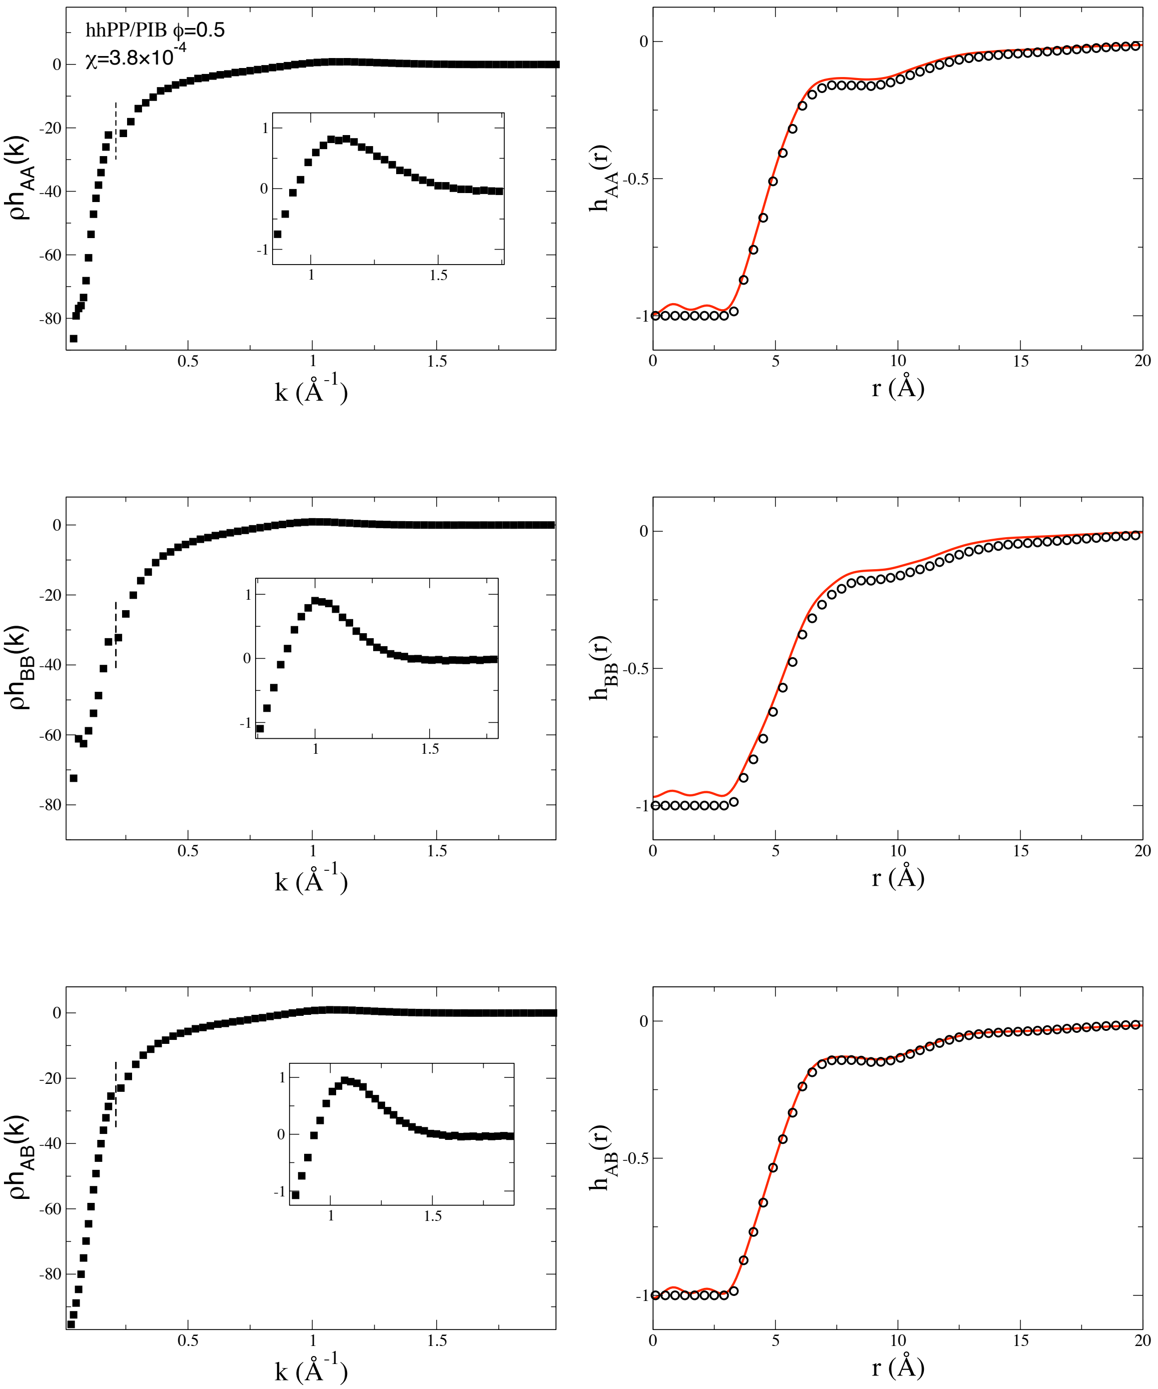


FIG. 3: Same as in Figure 1 except for a thermal mixture of hhPP/PIB at $T = 453K$, corresponding to a value of $\chi = 3.8 \times 10^{-4}$ in our mesoscale simulations.
